# Supplementary material for: Basins of Attraction for Chimera States
Source: arXiv:1507.01457 ancillary file (2016-02-15)
Supplement: Supplementary file 1 [file Supplementary_Video_Description.pdf]

# Supplement: Description of Supplementary Videos for Basins of Attraction for Chimera States

**Erik A. Martens**[a,b], **Mark J. Panaggio**[c,d], **Daniel M. Abrams**[d,e,f]

[a]Dept. of Biomedical Sciences, University of Copenhagen, Blegdamsvej 3, 2200 Copenhagen, Denmark

[b]Dept. of Mathematical Sciences, University of Copenhagen, Universitetsparken 5, 2200 Copenhagen, Denmark

[c]Mathematics Dept., Rose-Hulman Institute of Technology, Terre Haute, IN

[d]Dept. of Engineering Sciences and Applied Mathematics, Northwestern University, Evanston, IL

[e]Dept. of Physics and Astronomy, Northwestern University, Evanston, IL

[f]Northwestern Institute on Complex Systems, Northwestern University, Evanston, IL

E-mail: `erik.martens@ds.mpg.de`

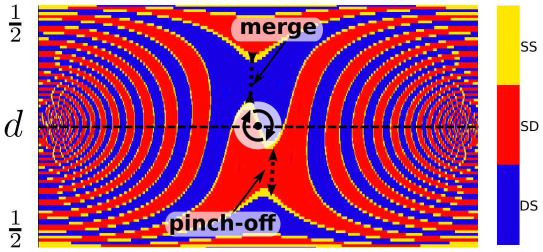


**Figure 1. Supplementary Video 1:** Destination maps as a function of $0.1 \leq s \leq 1$ ($A = 0.2, \beta = 0.025$). Even though $A = 0.2$ is fairly large with regards to our perturbative calculus, numerical results match the predicted motion qualitatively well. As $s$ increases from zero, basins merge and pinch-off in an alternating fashion, so that the basin boundaries rotate counter-clockwise about $R_0$ ($(d, \psi) = (0, 0)$). Once $s$ reaches $s_c \approx \sqrt{1 - A}$, this rotation stops, demonstrating that knowledge of the trajectory position in the $s = s_c$ plane is sufficient for determining the final fate of the trajectory. Download link here.

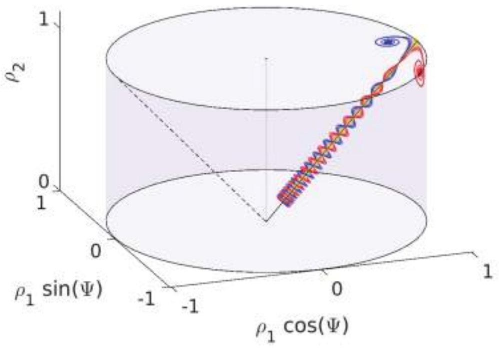


**Figure 2. Supplementary Video 2:** Twisting motion of trajectories in a double helical structure following the $R_0$-manifold ($A = 0.1, \beta = 0.025$). Initial conditions of 31 trajectories are equally spaced with $s = 0.1045, -0.0345 \leq d \leq 0.0345, \psi = 0$. Download link here.

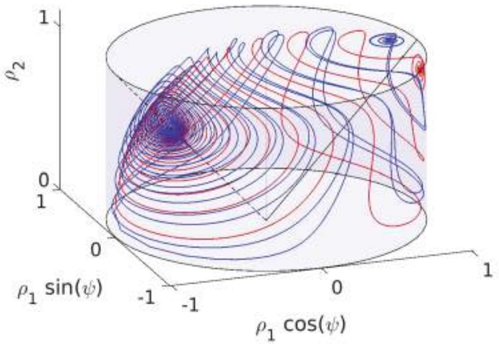


**Figure 3. Supplementary Video 3:** Twisting motion of trajectories in a double helical structure following the $R_\pi$ manifold ($A = 0.1, \beta = 0.025$). Initial conditions of the 3 trajectories are $s = 0.4487, d \in \{-0.6, -0.2, 0.6\} \times 10^{-3}, \psi = \pi$. Download link here.

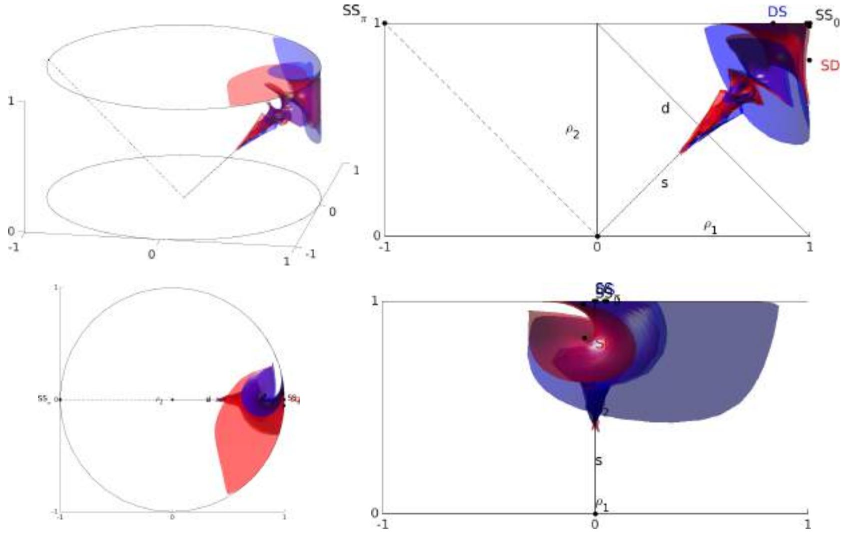


**Figure 4. Supplementary Video 4:** Three dimensional visualization of the separatrices emanating from the chimera saddle points near the $R_0$-manifold ($A = 0.1, \beta = 0.025$). Download link here.
